# Supplementary material for: ScaleQC: A Scalable Framework for Hybrid Computation on Quantum and Classical Processors
Source: arXiv:2207.00933 source file (2022-07-03)
Supplement: Supplementary file 1 [file Appendix.tex]

\appendix
\section{Appendix}
\subsection{Proof of Lemma~\ref{lemma:arbitrary_sampling}}\label{sec:lemma_arbitrary}
\begin{proof}
    The exact quantum state probability of state $j$ is given by:
    \begin{equation*}
        P_j=\sum_{k=1}^{4^K}\left(\otimes_{i=1}^{n_C}p_{i,k}\right)_j
    \end{equation*}
    
    For a particular $j$, $\forall t=1,\ldots,c$, define
    \begin{equation*}
        X_t=\left(\frac{\otimes_{i=1}^{n_C} p_{i,k_t}}{cq_{k_t}}\right)_j
    \end{equation*}
    
    Thus,
    \begin{eqnarray*}
    \mathbb{E}[X_t]&=&\sum_{k=1}^{4^K}q_{k}\left(\frac{\otimes_{i=1}^{n_C} p_{i,k}}{cq_k}\right)_j\\
    &=&\frac{1}{c}\sum_{k=1}^{4^K}\left(\otimes_{i=1}^{n_C} p_{i,k}\right)_j
    \end{eqnarray*}
    
    And
    \begin{eqnarray*}
    \mathbb{E}[X_t^2]&=&\sum_{k=1}^{4^K}q_{k}\left(\frac{\otimes_{i=1}^{n_C} p_{i,k}}{cq_k}\right)_j^2\\
    &=&\frac{1}{c^2}\sum_{k=1}^{4^K}\frac{\left(\otimes_{i=1}^{n_C} p_{i,k}\right)_j^2}{q_k}
    \end{eqnarray*}
    
    Hence by construction, Equation~\ref{eq:arbitrary_expectation} follows:
    \begin{eqnarray*}
    \mathbb{E}[\widetilde{P}_j]&=&\sum_{t=1}^c\mathbb{E}[X_t]\\
    &=&\sum_{k=1}^{4^K}\left(\otimes_{i=1}^{n_C} p_{i,k}\right)_j\\
    &=&P_j
    \end{eqnarray*}
    
    Since we are taking $c$ independent random variables,
    \begin{eqnarray*}
    \text{Var}[\widetilde{P}_j]&=&\sum_{t=1}^c\text{Var}[X_t]\\
    \text{Var}[X_t]&=&\mathbb{E}[X_t^2]-\mathbb{E}[X_t]^2\\
    &=&\frac{1}{c^2}\sum_{k=1}^{4^K}\frac{\left(\otimes_{i=1}^{n_C} p_{i,k}\right)_j^2}{q_k}-\frac{1}{c^2}P_j^2\\
    \end{eqnarray*}
    Hence Equation~\ref{eq:arbitrary_variance} follows.
    
    Note that the expectation of the approximation error is given by
    \begin{eqnarray*}
    \mathbb{E}[\epsilon]&=&\sum_{j=1}^{2^n}\mathbb{E}\left[(P_j-\widetilde{P}_j)^2\right]\\
    &=&\sum_{j=1}^{2^n}\text{Var}\left[(P_j-\widetilde{P}_j)\right]+\mathbb{E}\left[(P_j-\widetilde{P}_j)\right]^2\\
    &=&\sum_{j=1}^{2^n}\text{Var}\left[\widetilde{P}_j\right]
    \end{eqnarray*}
    Substituting Equation~\ref{eq:arbitrary_variance} gives:
    \begin{eqnarray*}
    \mathbb{E}[\epsilon]&=&\sum_{j=1}^{2^n}\left[\frac{1}{c}\sum_{k=1}^{4^K}\frac{\left(\otimes_{i=1}^{n_C} C_{i,k}\right)_j^2}{p_k}-\frac{1}{c}P_j^2\right]\\
    &=&\frac{1}{c}\sum_{k=1}^{4^K}\frac{|\otimes_{i=1}^{n_C} C_{i,k}|^2}{p_k}-\frac{1}{c}|P|^2\\
    &=&\frac{1}{c}\sum_{k=1}^{4^K}\frac{1}{p_k}\prod_{i=1}^{n_C}|C_{i,k}|^2-\frac{1}{c}|P|^2
    \end{eqnarray*}
    Hence Equation~\ref{eq:arbitrary_error} follows.
\end{proof}

\subsection{Proof of Lemma~\ref{lemma:optimal_sampling}}\label{sec:lemma_optimal}
\begin{proof}
    Define
    \begin{equation}
        f(q_1,\ldots,q_{4^K})=\sum_{k=1}^{4^K}\frac{1}{q_k}\prod_{i=1}^{n_C}|p_{i,k}|^2\label{eq:probability_function}
    \end{equation}
    Note that minimizing Equation~\ref{eq:probability_function} (subject to that the $q_k$s form a valid probability distribution) is the same as minimizing Equation~\ref{eq:arbitrary_error}.
    Introduce the Lagrange multiplier method:
    \begin{eqnarray*}
    \nabla f(q_1,\ldots,q_{4^K})&=&-\lambda\nabla\left[\sum_{k=1}^{4^K}q_k-1\right]\\
    \frac{\partial f}{\partial q_k}&=&-\lambda\\
    -\frac{1}{q_k^2}\prod_{i=1}^{n_C}|p_{i,k}|^2&=&-\lambda\\
    q_k&=&\frac{\prod_{i=1}^{n_C}|p_{i,k}|}{\sqrt{\lambda}}
    \end{eqnarray*}
    Solve for $\lambda$:
    \begin{eqnarray*}
    \sum_{k=1}^{4^K}\frac{\prod_{i=1}^{n_C}|p_{i,k}|}{\sqrt{\lambda}}&=&1\\
    \sqrt{\lambda}&=&\sum_{k=1}^{4^K}\prod_{i=1}^{n_C}|p_{i,k}|
    \end{eqnarray*}
    Therefore Equation~\ref{eq:optimal_probability} follows.
    Substituting Equation~\ref{eq:optimal_probability} into Equation~\ref{eq:arbitrary_error} hence gives the minimum expected approximation error in Equation~\ref{eq:optimal_error}.
\end{proof}
